# Supplementary material for: Lean Census: A Distributional Analysis of AI-Generated Lean Code
Source: arXiv:2611.28430 source file (2026-11-21)
Supplement: Supplementary file 1 [file appendix-figures.tex]

\begin{figure}[H]\centering
\includegraphics[width=\linewidth]{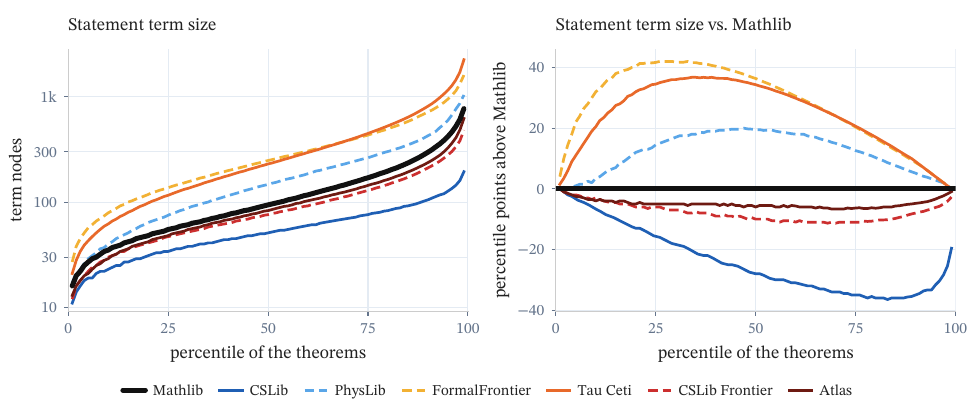}
\caption{Statement term size. Distinct nodes of the elaborated type, so formatting and notation play no part.}
\label{fig:type_dag}
\end{figure}

\begin{figure}[H]\centering
\includegraphics[width=\linewidth]{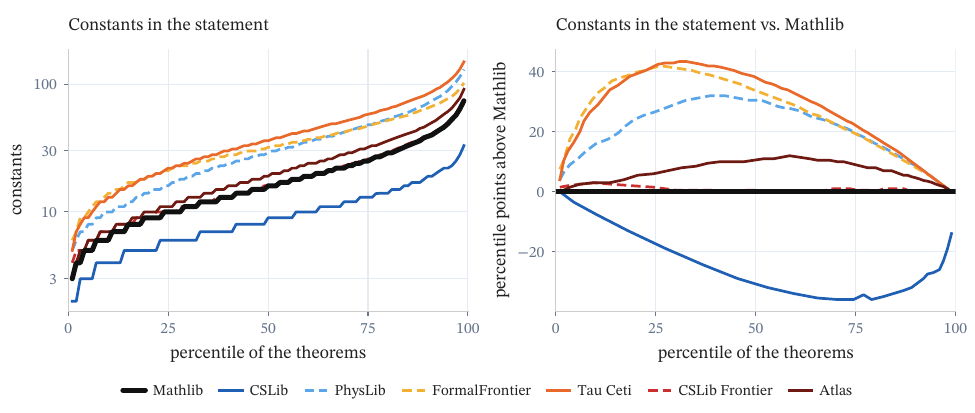}
\caption{Constants in the statement. Distinct declarations the elaborated statement mentions.}
\label{fig:out_stmt}
\end{figure}

\begin{figure}[H]\centering
\includegraphics[width=\linewidth]{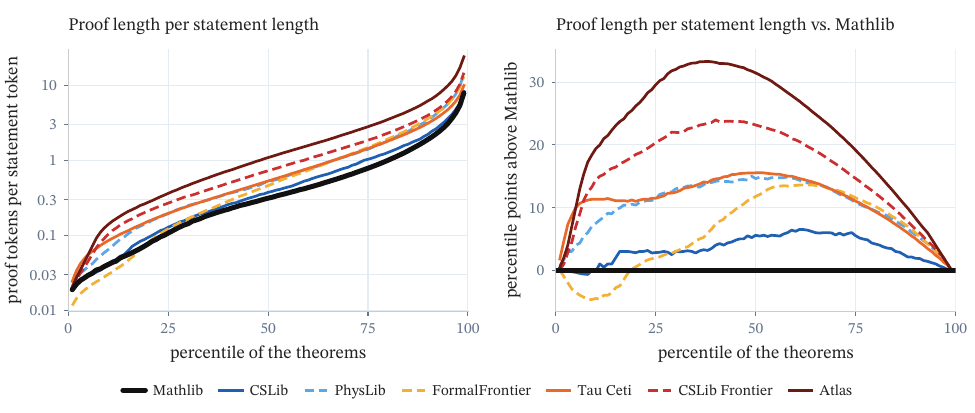}
\caption{Proof length per statement length. Proof tokens divided by statement tokens.}
\label{fig:body_per_stmt}
\end{figure}

\begin{figure}[H]\centering
\includegraphics[width=\linewidth]{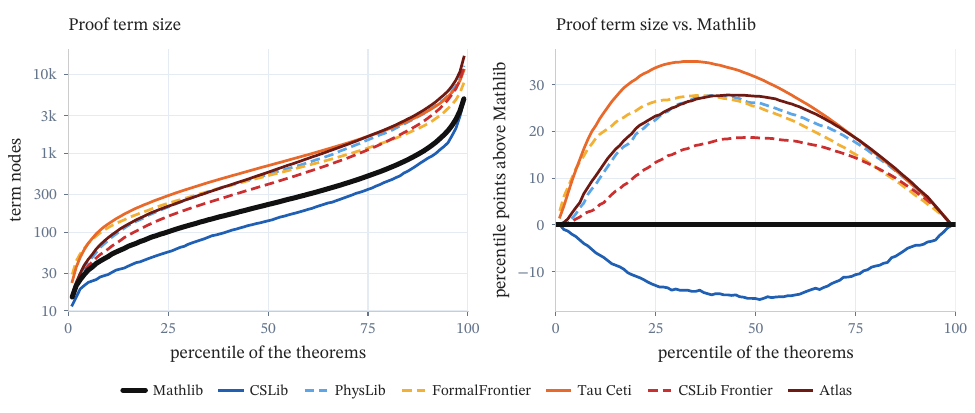}
\caption{Proof term size. Distinct nodes of the elaborated proof, with Lean's auxiliary terms folded in.}
\label{fig:value_dag_owned}
\end{figure}

\begin{figure}[H]\centering
\includegraphics[width=\linewidth]{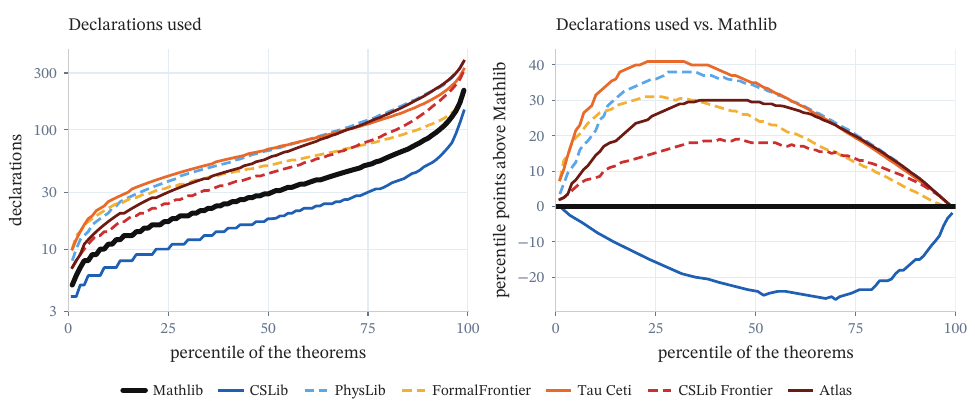}
\caption{Declarations used. Distinct declarations the statement and proof refer to.}
\label{fig:out_all}
\end{figure}

\begin{figure}[H]\centering
\includegraphics[width=\linewidth]{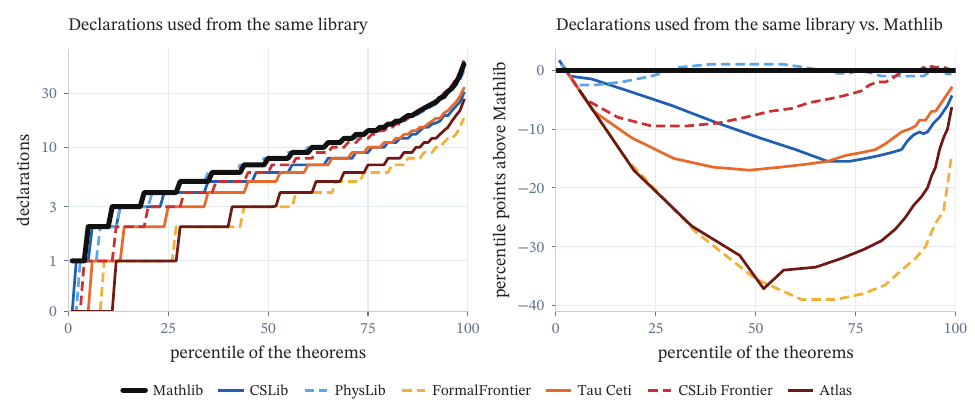}
\caption{Declarations used from the same library. Distinct declarations of the same library that the statement and proof refer to. For Mathlib, the library is the top-level area.}
\label{fig:out_same}
\end{figure}

\begin{figure}[H]\centering
\includegraphics[width=\linewidth]{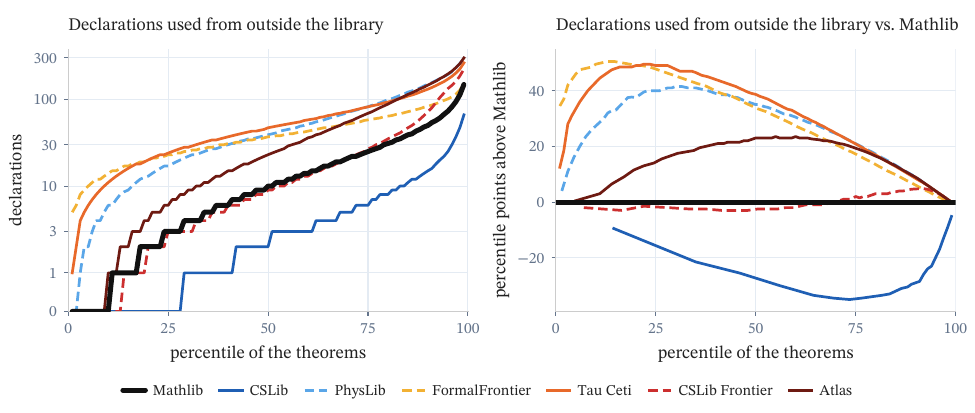}
\caption{Declarations used from outside the library. Distinct declarations outside the library, mostly from Mathlib, that the statement and proof refer to.}
\label{fig:out_upstream}
\end{figure}

\begin{figure}[H]\centering
\includegraphics[width=\linewidth]{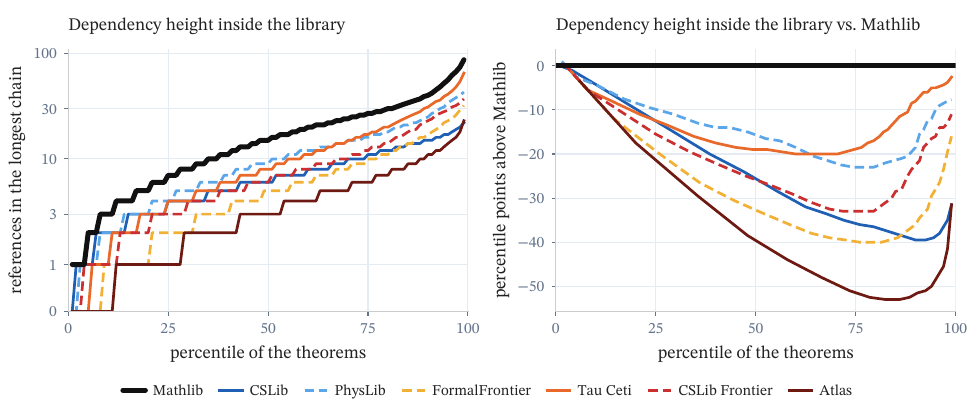}
\caption{Dependency height inside the library. Longest chain of references that stays inside the library.}
\label{fig:depth_own}
\end{figure}

\begin{figure}[H]\centering
\includegraphics[width=\linewidth]{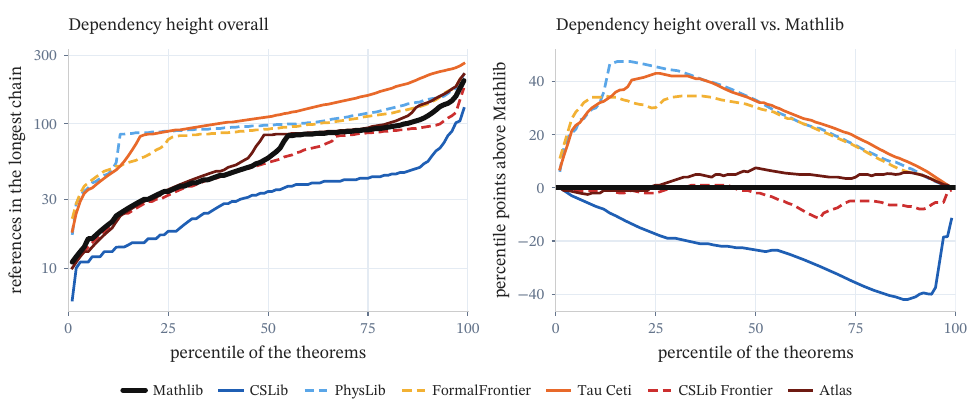}
\caption{Dependency height overall. Longest chain of references down to the axioms.}
\label{fig:depth_all}
\end{figure}

\begin{figure}[H]\centering
\includegraphics[width=\linewidth]{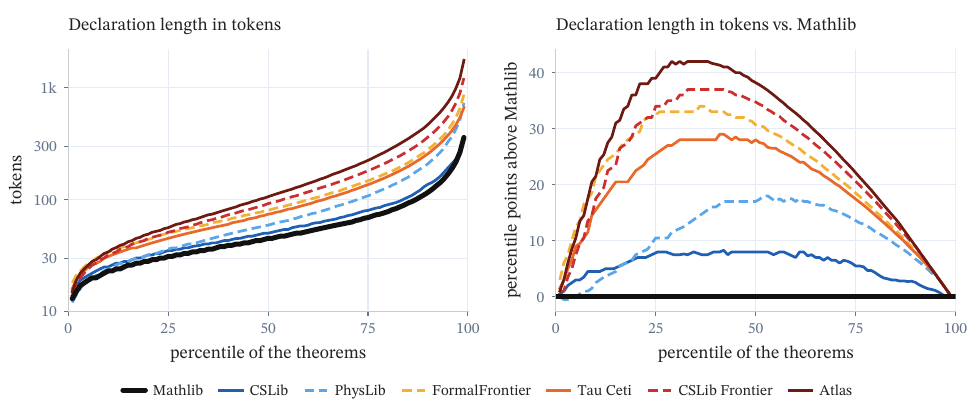}
\caption{Declaration length in tokens. Statement and proof together, the source-token analogue of the wrapped length of \citet{aksenov2026compression}.}
\label{fig:tokens}
\end{figure}

\begin{figure}[H]\centering
\includegraphics[width=\linewidth]{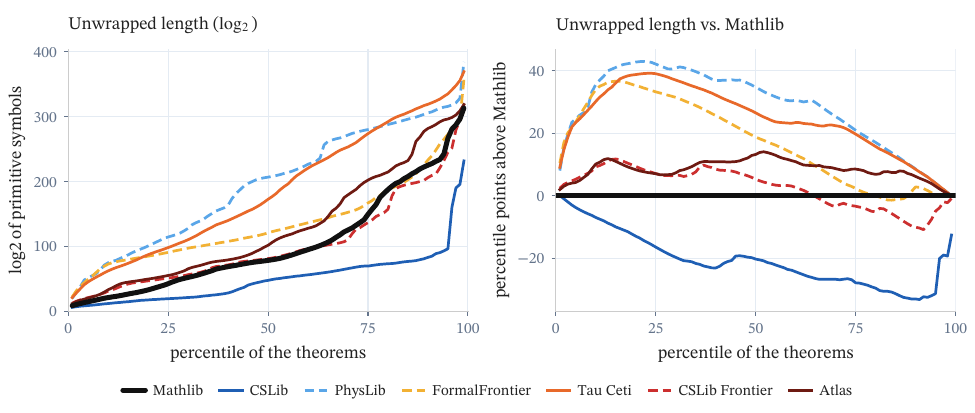}
\caption{Unwrapped length ($\log_2$). Primitive symbols after expanding every reference, core library included. \citet{aksenov2026compression} instead treat the core library as primitive and handle cycles differently.}
\label{fig:unwrapped_log2}
\end{figure}

\begin{figure}[H]\centering
\includegraphics[width=\linewidth]{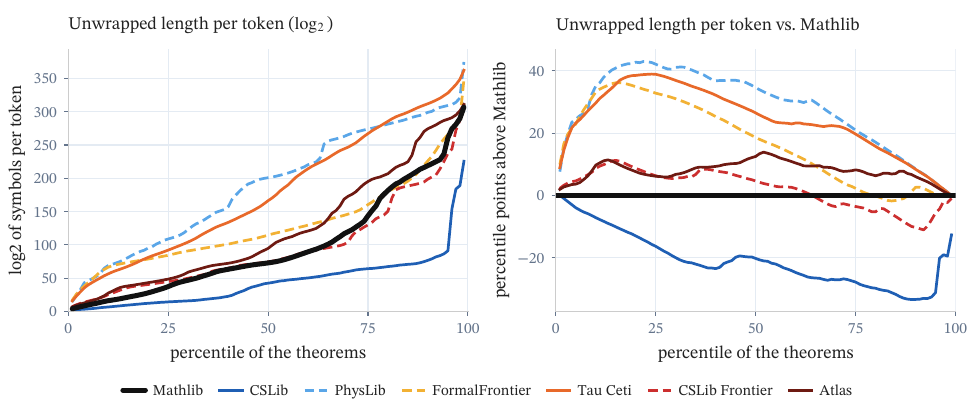}
\caption{Unwrapped length per token ($\log_2$). Unwrapped length divided by declaration length in tokens, a variant of the compression measure of \citet{aksenov2026compression}, unrelated to the file compression of Appendix~\ref{app:inventory}.}
\label{fig:taste_log2}
\end{figure}
